# Supplementary material for: The Resource Problem of Using Linear Layer Leakage Attack in Federated Learning
Source: arXiv:2303.14868 source file (2023-03-27)
Supplement: Supplementary file 1 [file 5_additional_discussions.tex]

% \subsection{FedAVG}
\iffalse
Over the course of a single FedAVG round, the parameters in the model will shift slightly. Since we use the same FC layer leakage methodology from Robbing the Fed, our application to FedAVG for the weights and biases of the layer follow the prior work. We also add a convolutional layer to the method. For this case, the parameters will change slightly when training each local mini-batch. These changes in the parameters are small and result in a minimal degradation of image quality~\cite{our2022mandrake}. We note that the size of the FC layer should be large enough for the size of the local client dataset in order to maintain a high leakage rate.
\fi

Unlike the gradients of the FC layers, the gradients of the convolutional layer are not necessary for the data reconstruction attack. A malicious server can then send a maliciously crafted model which would freeze the parameters of the convolutional layer to prevent changes from occurring over the local iterations of FedAVG. 

\iffalse
\subsection{Defenses}
Model architecture or parameter manipulation is much more difficult for clients in cross-device FL. As a result, clients must consider alternatives for privacy-preserving defenses. As discussed in this paper, secure aggregation (SA), or any other similar defense such as secure shuffling~\cite{kairouz2021advances}, is ineffective against linear layer leakage methods.

Differential privacy (DP) is also a commonly used method to preserve client data privacy in FL~\cite{dwork2014algorithmic, wei2020federated}. Particularly, if a client injects some noise into their model update, even a perfect reconstruction attack cannot recover the inputs without noise. This still holds true for linear layer leakage attacks. However, DP will hurt the model performance. Additionally, since the clients have no knowledge of when an attack will occur, they will be forced to apply DP for each participating training round. 
\fi
